# Supplementary material for: Discrete and Continuous Wigner Functions in Open Quantum Systems: Non-Markovian and Thermodynamic Effects
Source: arXiv:2605.29717 source file (2026-05-28)
Supplement: Supplementary file 3 [file AppendixTemplate.tex]

% Appendix Template
\chapter{Appendix X} % Main appendix title

\label{AppendixX} % Change X to a consecutive letter; for referencing this appendix elsewhere, use \ref{AppendixX}
